# Supplementary material for: Spin wavepacket propagation in quasi-2D antiferromagnets
Source: arXiv:2212.03261 source file (2022-12-06)
Supplement: Supplementary file 2 [file main_SI_appendices.tex]

\documentclass{article}
\pdfoutput=1
\usepackage[utf8]{inputenc}
\usepackage{pdfpages}
\begin{document}
\includepdf[pages=-]{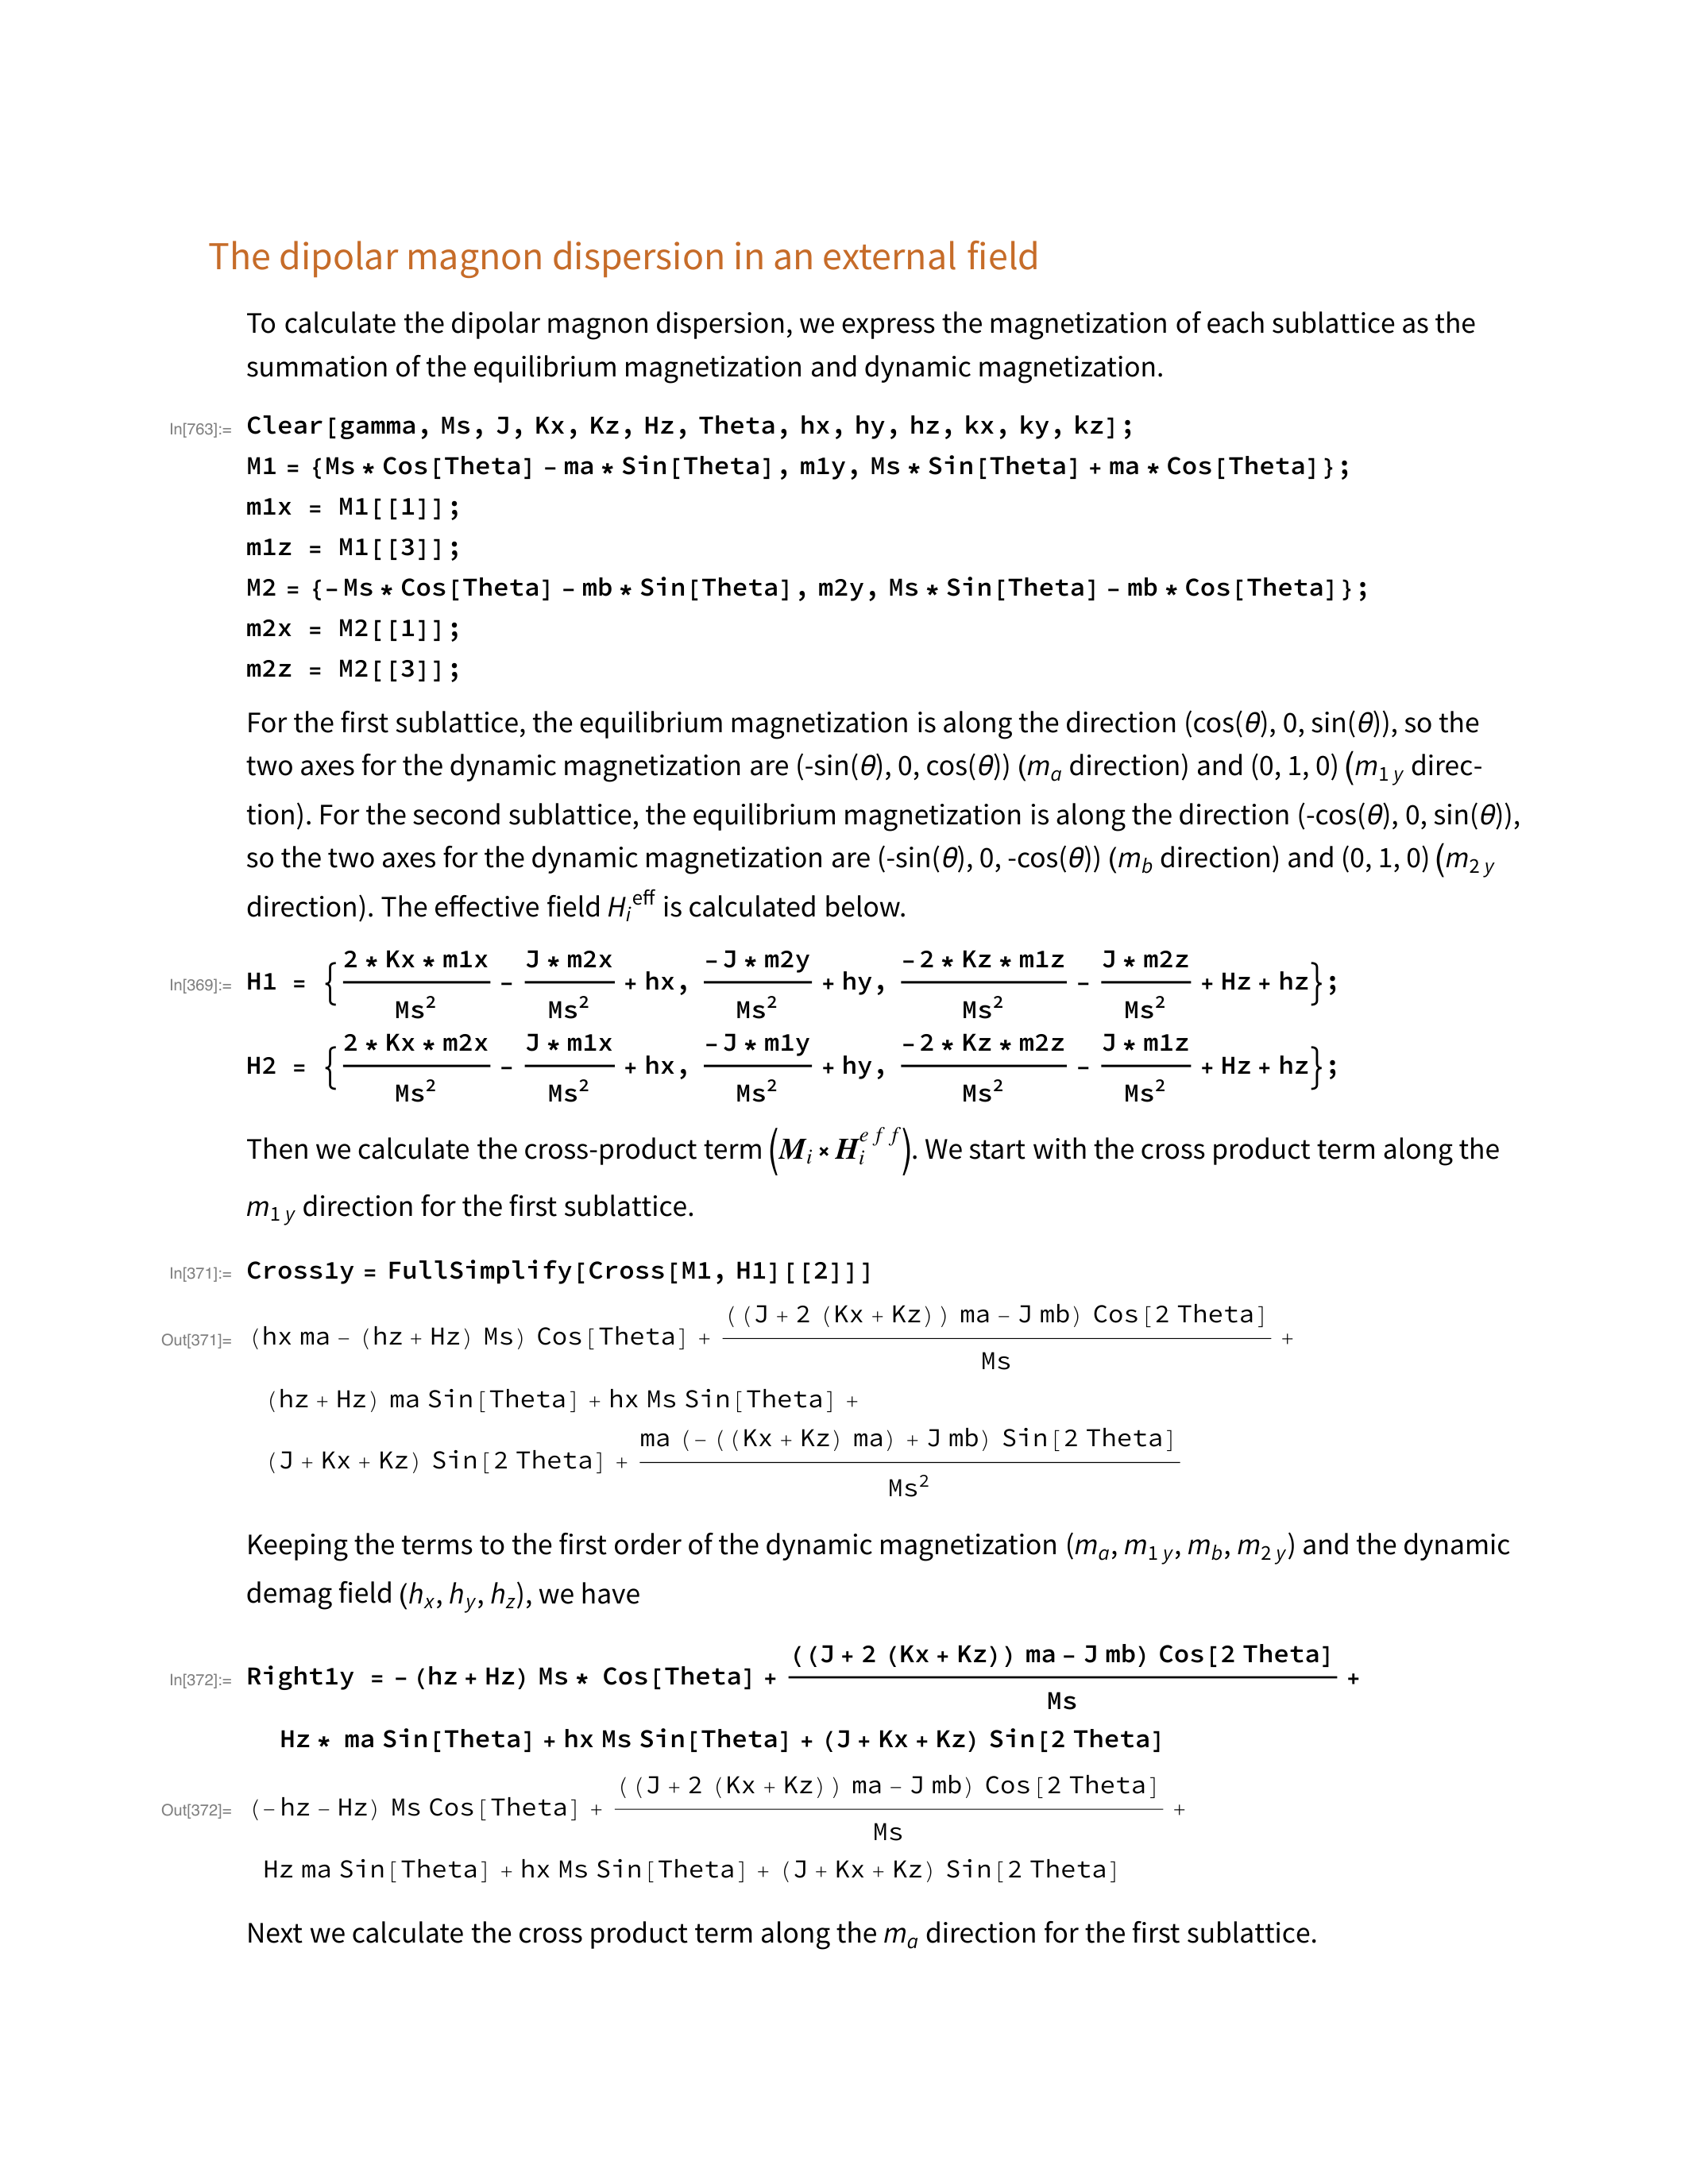}
\includepdf[pages=-]{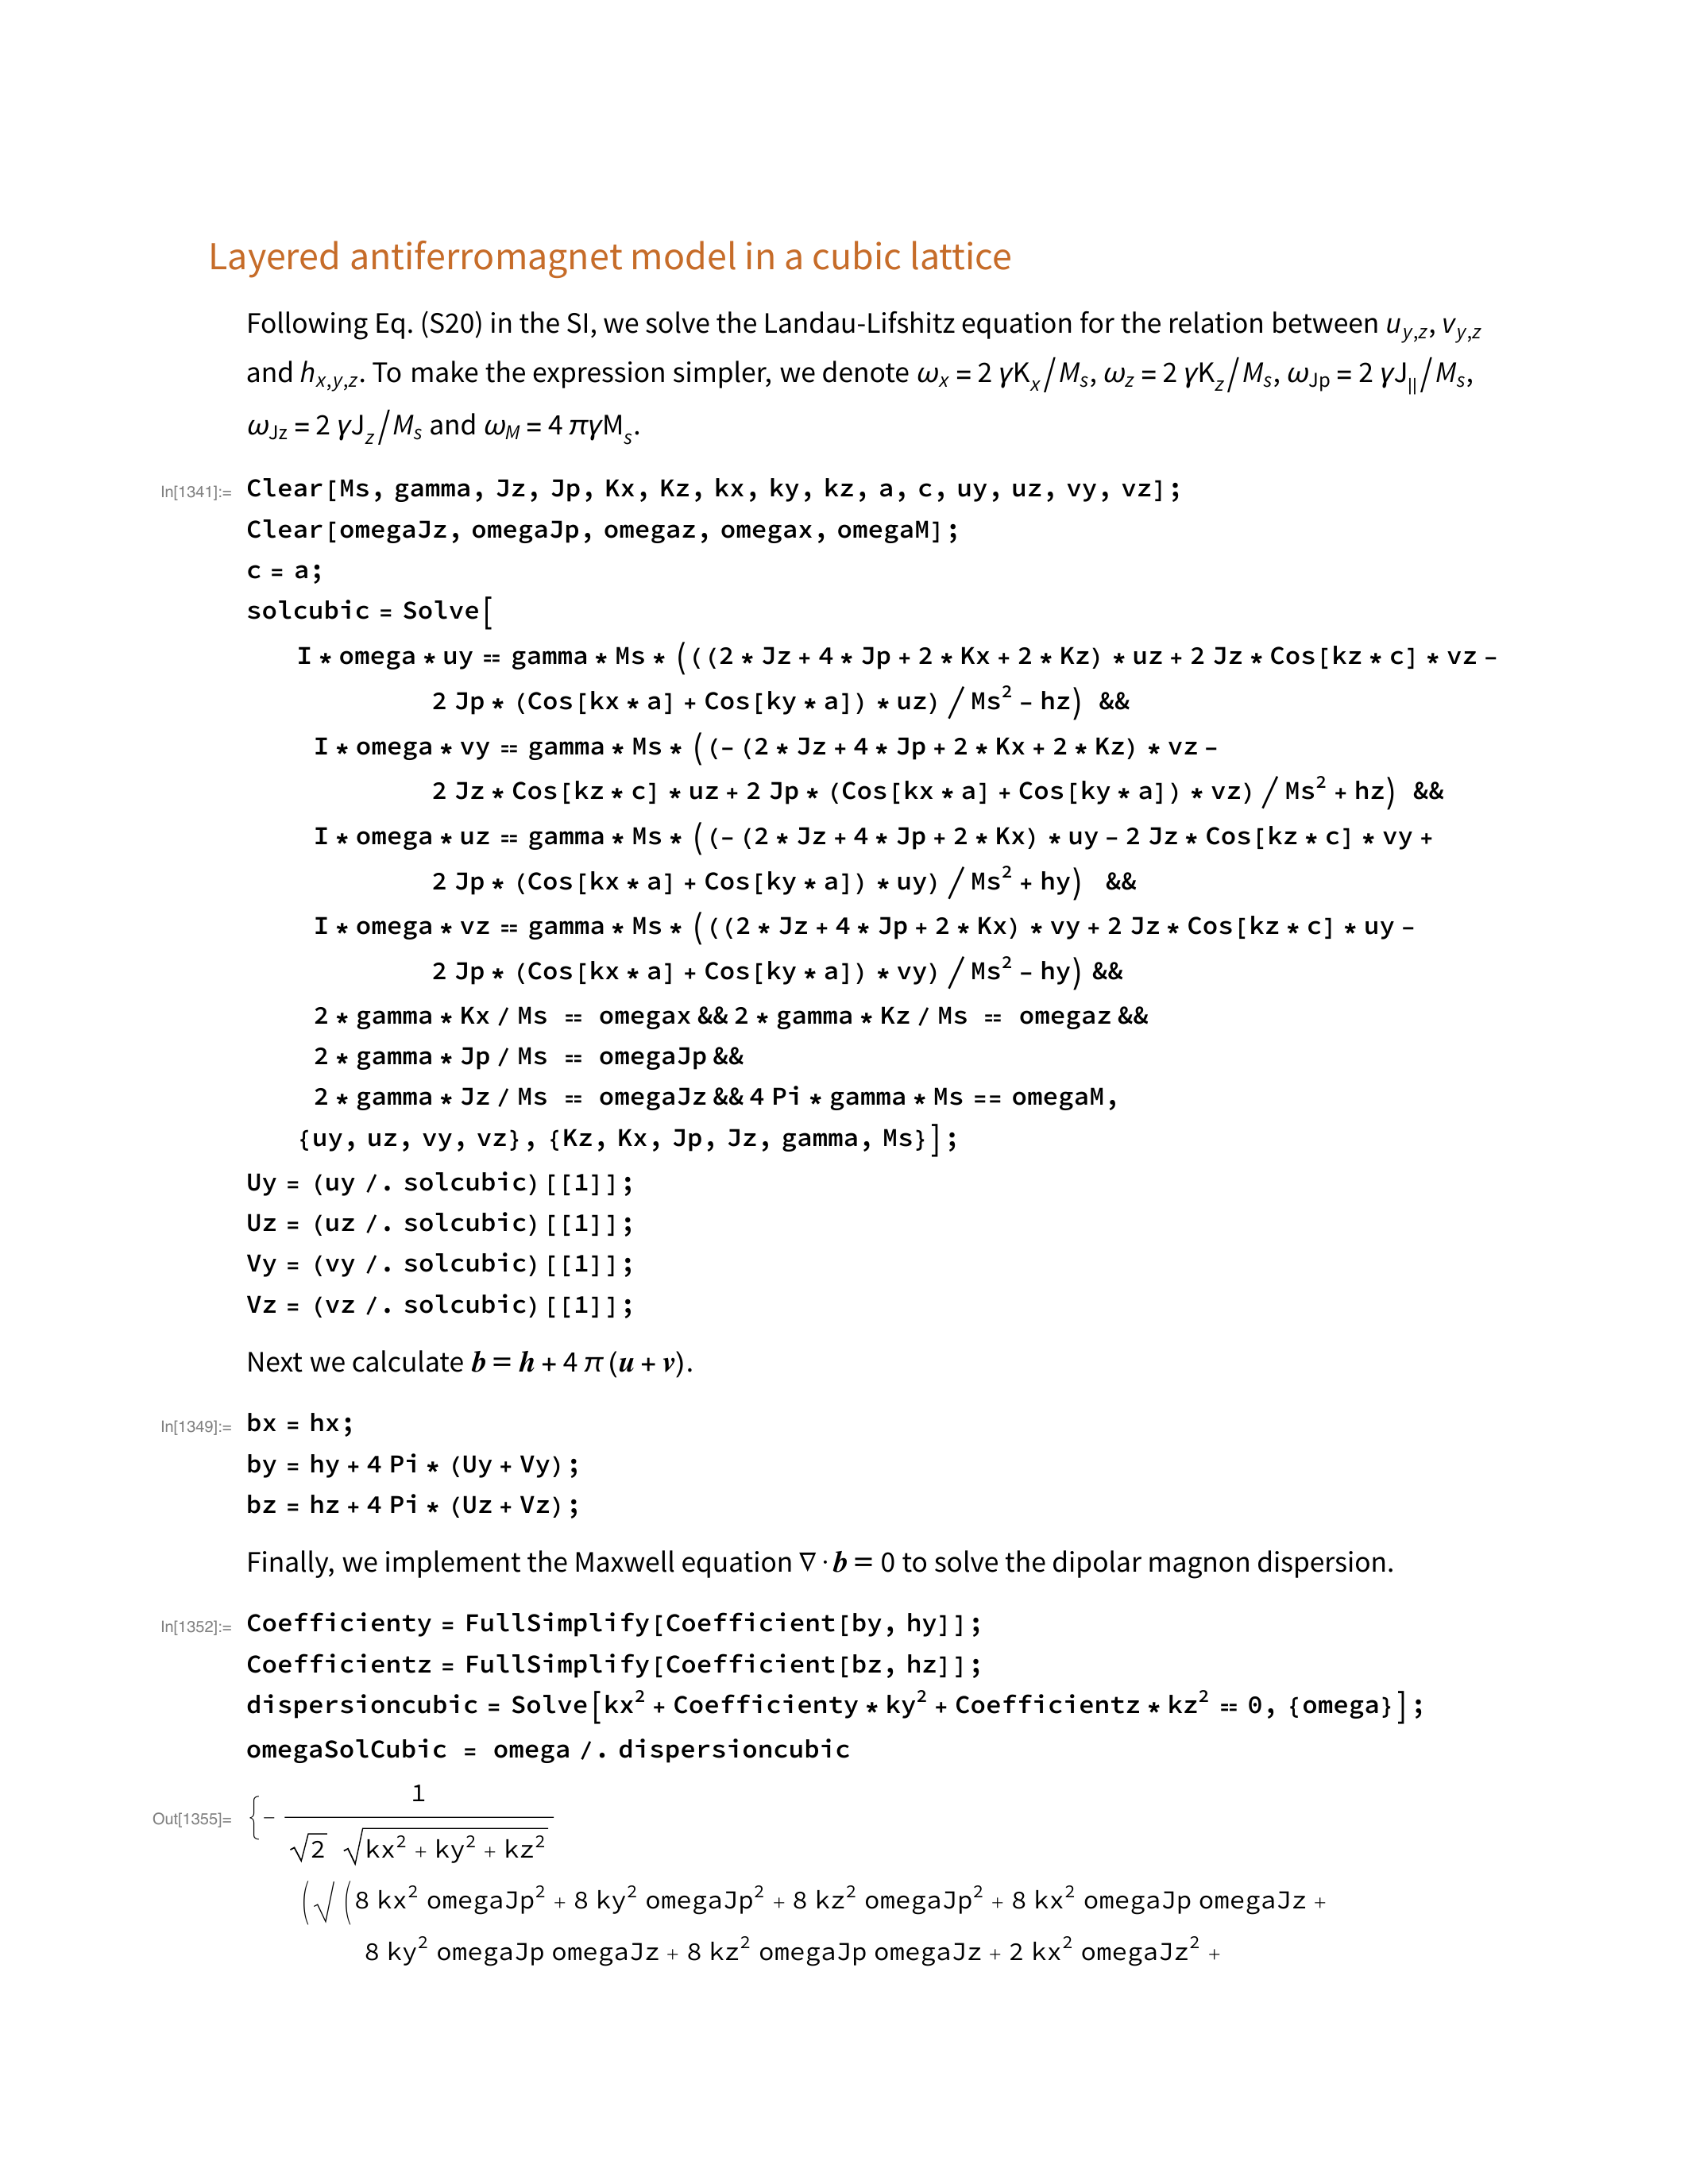}
\end{document}
